# Supplementary material for: Optical and Transport Properties of Plasma Mixtures from Ab Initio Molecular Dynamics
Source: arXiv:2404.07800 source file (2024-04-11)
Supplement: Supplementary file 1 [file supplemental.pdf]

# Supplemental Materials : Optical and Transport Properties of Plasma Mixtures from *Ab Initio* Molecular Dynamics

Alexander J. White, Galen T. Craven, Vidushi Sharma, and Lee A. Collins

*Theoretical Division, Los Alamos National Laboratory, Los Alamos, New Mexico 87544*

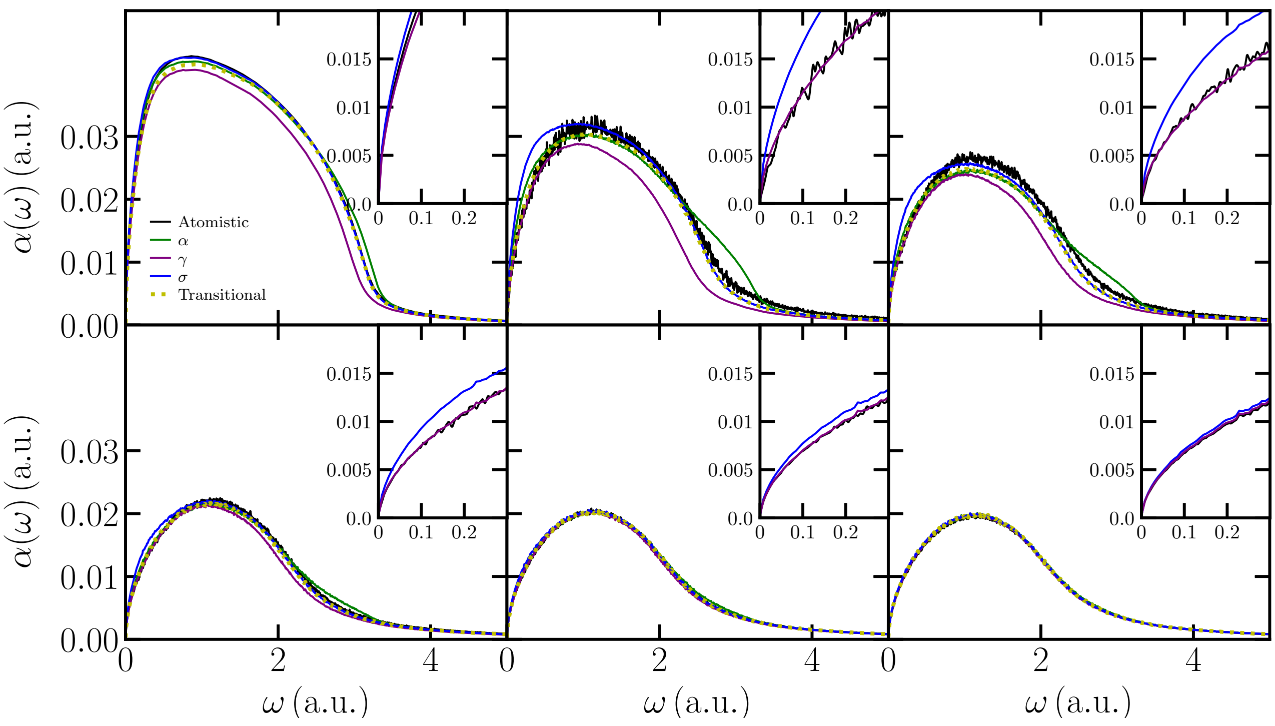


FIG. 1. Isodensity CH mixtures at 10 g/cc 10 eV. Black line - atomistic calculation of mixture absorbance, Green line - volumetrically mixed absorbance, Purple line - absorbance calculated from volumetrically mixed effective scattering rates, blue-line absorbance calculated from volumetrically mixed AC conductivity. Top left (1% C), Top center (10% C), Top right (25% C), bottom left (50% C), bottom center (75% C), bottom right (90% C)

Concentration dependent absorption and reflectivity plots for the isodensity case (Fig 1 and 2) and the isobaric case (Fig 3 and 4). Similar to Fig XX of the main text.

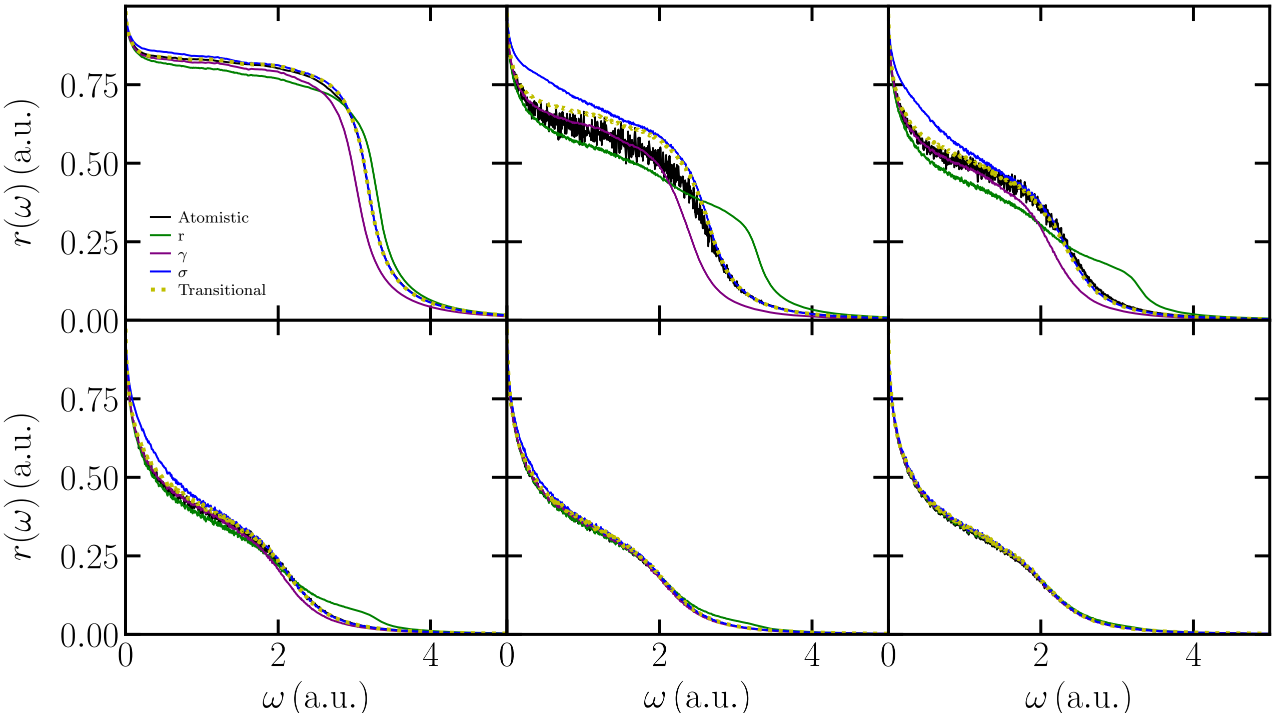


FIG. 2. Isodensity CH mixtures at 10 g/cc 10 eV. Black line - atomistic calculation of mixture resistivity, Green line - volumetrically mixed resistivity, Purple line - resistivity calculated from volumetrically mixed effective scattering rates, blue-line resistivity calculated from volumetrically mixed AC conductivity. Top left (1% C), Top center (10% C), Top right (25% C), bottom left (50% C), bottom center (75% C), bottom right (90% C)

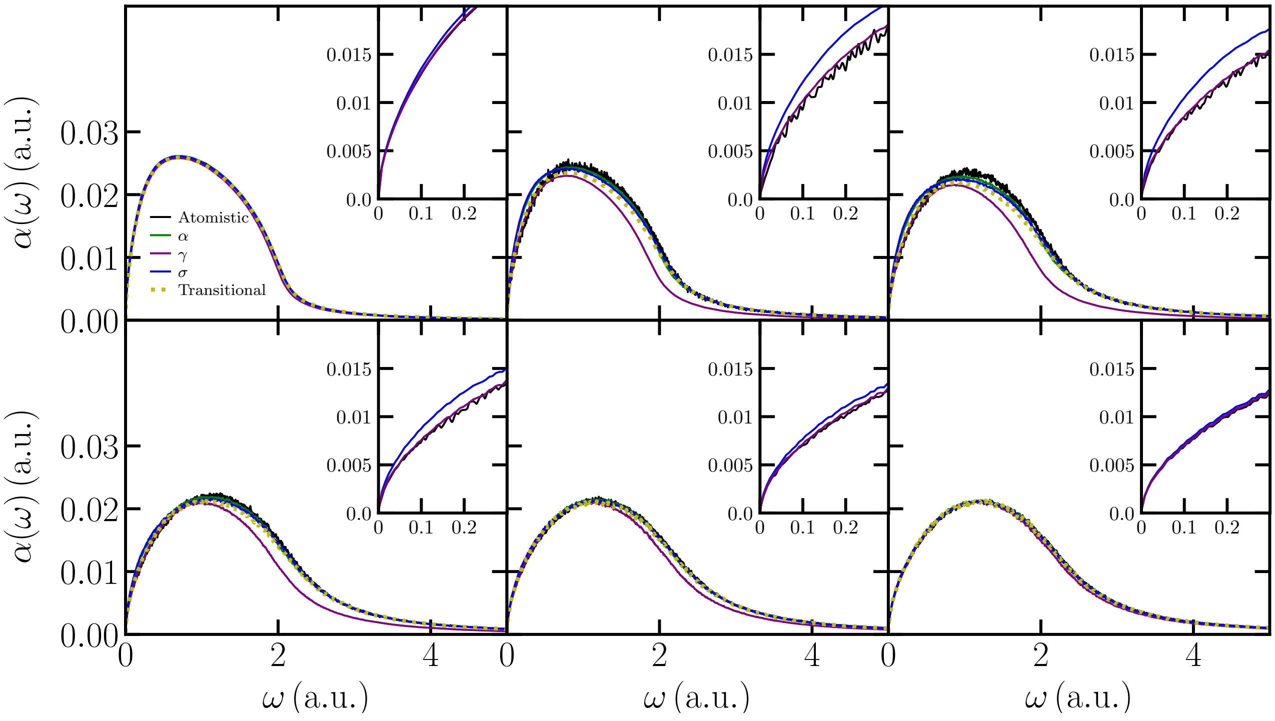


FIG. 3. Isobaric CH mixtures at ∼ 5580 GPa electronic pressure. Black line - atomistic calculation of mixture absorbance, Green line - volumetrically mixed absorbance, Purple line - absorbance calculated from volumetrically mixed effective scattering rates, blue-line absorbance calculated from volumetrically mixed AC conductivity. Top left (1% C), Top center (10% C), Top right (25% C), bottom left (50% C), bottom center (75% C), bottom right (90% C)

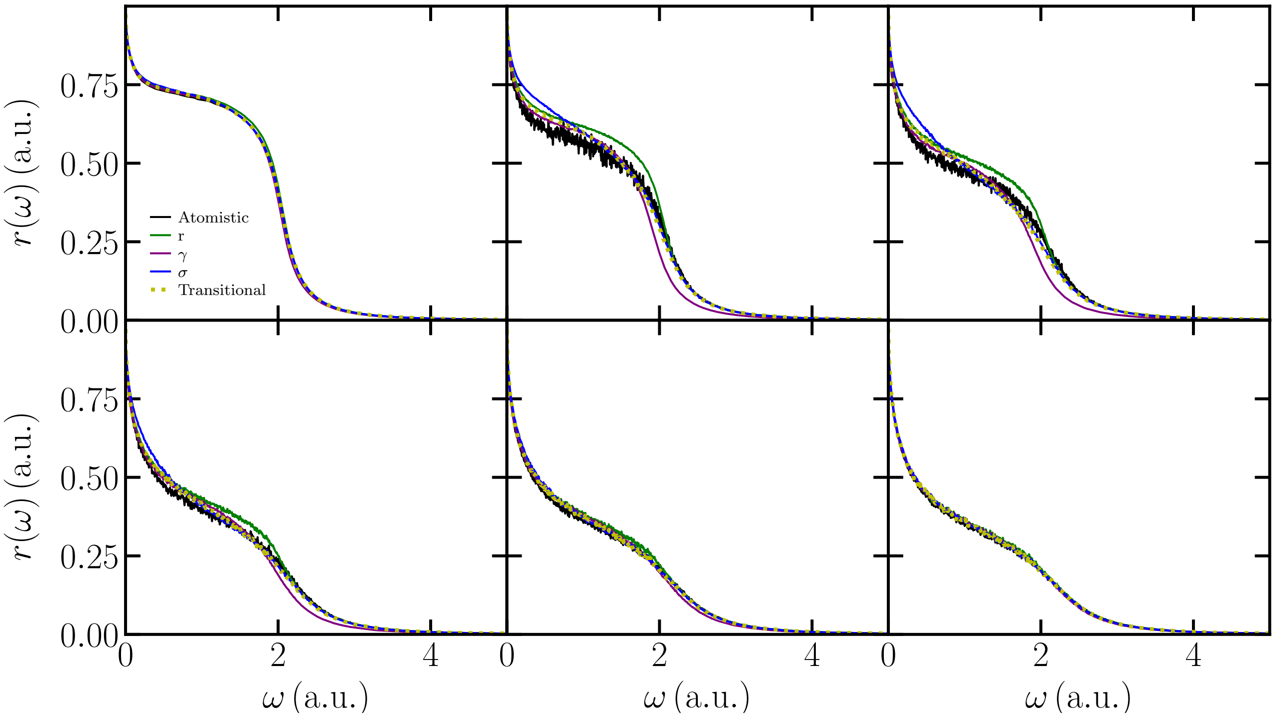


FIG. 4. Isobaric CH mixtures at ∼ 5580 GPa electronic pressure. Black line - atomistic calculation of mixture resistivity, Green line - volumetrically mixed resistivity, Purple line - resistivity calculated from volumetrically mixed effective scattering rates, blue-line resistivity calculated from volumetrically mixed AC conductivity. Top left (1% C), Top center (10% C), Top right (25% C), bottom left (50% C), bottom center (75% C), bottom right (90% C)
